# Supplementary material for: Excitatory and inhibitory interactions affect the balance of chorus activity and energy efficiency in the aggregation of male frogs: Theoretical study using a hybrid dynamical model
Source: arXiv:2111.02640 source file (2021-11-04)
Supplement: Supplementary file 1 [file SI_20211104.pdf]

# Supplementary Information: Excitatory and inhibitory interactions affect the balance of chorus activity and energy efficiency in the aggregation of male frogs: Theoretical study using a hybrid dynamical model

Ikkyu Aihara[1,*], Daichi Kominami[2], Yushi Hosokawa[2], Masayuki Murata[2]

**1 Faculty of Engineering, Information and Systems, University of Tsukuba, Ibaraki 305-8573, Japan**

**2 Graduate School of Information Science and Technology, Osaka University, Osaka 565-0871, Japan**

**∗ E-mail: aihara@cs.tsukuba.ac.jp**

| Parameter | Value | Equation including the parameter | Brief explanation |
|---|---|---|---|
| $\omega_n$ | $2\pi/0.306$ | Equation (1) | An intrinsic angular velocity of a phase oscillator model (Equation (1)). In the model, $2\pi/\omega$ represents an intrinsic inter-call interval of the $n$th frog. This parameter was fixed at the same value with our previous study [1]. |
| $r_{\mathrm{acoustic}}$ | 100.0 | Equation (1) | Acoustic interaction range among male frogs. Because the calls of male frogs are loud and propagate in space, we fixed this parameter at a large value comparable to the size of their breeding site. |
| $K_{nm}$ | 0.20 | Equation (4) | Coupling strength between the $n$th frog and $m$th frog in a phase oscillator model. This parameter was fixed at the same value with our previous study [1] to qualitatively reproduce multiple alternating chorus patterns of male frogs (e.g., anti-phase synchronization of two frogs, tri-phase synchronization of three frogs, and clustered synchronization of three frogs). |
| $k$ | 0.18 | Equation (4) | Coupling strength of the second order component in a phase oscillator model. This parameter was fixed at the same value with our previous study [1] to reproduce the alternating chorus patterns of male frogs. |
| $\alpha$ | $0.12\omega/2\pi$ | Equation (6) | Recovery rate of physical fatigue in a resting state or a satellite state. This parameter was fixed at the same value with our previous study [1] to reproduce collective transition between a calling state and a resting state. |
| $\beta_{\mathrm{fatigue}}$ | 0.50 | Equations (9) and (11) | Steepness of logistic functions that affects the probability of the transition between a calling state and a resting state depending on physical fatigue. This parameter was fixed at the same value with our previous study [1] to reproduce the collective transition between a calling state and a resting state. |
| $\Delta T$ | 25.53/0.306 | Equations (9) and (11) | Representative call number that each frog produces within a single bout. This parameter was fixed at the same value with our previous study [1] to reproduce the collective transition between a calling state and a resting state. |
| $\beta_{\mathrm{energy}}$ | 0.01 | Equation (12) | Steepness of a logistic function that affects the probability of the transition from a resting state to a calling state depending on remaining energy. This parameter was fixed at the same value with our previous study [1] to reproduce the collective transition between a calling state and a resting state. |

**Table S1.** Parameter values used for numerical simulations.

| Parameter | Value | Equation including the parameter | Brief explanation |
|---|---|---|---|
| $p_{\text{low}}$ | 0.01 | Equation (13) | The lower value of a discrete function that affects the probability of the transition from a resting state to a calling state depending on the existence of calling neighbors. This parameter was fixed at the same value with our previous study [1] to reproduce the collective transition between a calling state and a resting state. |
| $p_{\text{high}}$ | 0.80 | Equation (13) | The higher value of a discrete function that affects the probability of the transition from a resting state to a calling state depending on the existence of calling neighbors. This parameter was fixed at the same value with our previous study [1] to reproduce the collective transition between a calling state and a resting state. |
| $\beta_{\text{satellite}}$ | Varied | Equations (15) and (17) | Steepness of logistic functions that describe the probability of the transition between a resting state and a satellite state depending on relative attractiveness (the difference of call number included in the adjacent calling bout) to the nearest neighbor. We varied the value of this parameter because it dominantly affects the probability of the transition but we could not accurately quantify the value from empirical data. |
| $\Delta N$ | Varied | Equations (15) and (17) | Threshold of the relative attractiveness beyond which the transition between a resting state and a satellite state is induced at high probability. We varied the value of this parameter because it dominantly affects the probability of the transition but we could not accurately quantify the value from empirical data. |
| $T_{\text{max}}$ | $1.2\Delta T$ | N/A | The maximum value of physical fatigue. This parameter was fixed at the same value with our previous study [1]. |
| $E_{\text{max}}$ | 3878 | N/A | The maximum value of energy. This parameter was fixed at the same value with our previous study [1]. |

**Table S2.** (continued) Parameter values used for numerical simulations.

| Parameter | Value | Equation including the parameter | Brief explanation |
|---|---|---|---|
| $r_{\text{satellite}}$ | 0.4 | N/A | The distance within which a calling frog is recognized as the target of satellite behavior by his nearest neighbor. We fixed this parameter at the small value within which a satellite male can intercept a female attracted to the caller. |
| $t_{\text{update}}$ | 3.5 | N/A | Time interval at which each frog stochastically updates his state. This parameter was fixed at the same value with our previous study [1]. |
| $t_{\text{reset}}$ | 1000.0 | N/A | Time interval at which a satellite male resets the attractiveness of his nearest neighbor. In our model, a male frog cannot start calling again when his energy is empty. In such a case, their competitor is very likely starts calling again if he has enough energy. In fact, empirical studies showed that the removal of a calling male induce the calling behavior of a satellite male [2]. To reproduce this feature, we fix the parameter at larger value than the duration of a representative calling bout and also the duration of silence period between successive calling bouts. |

**Table S3.** (continued) Parameter values used for numerical simulations.

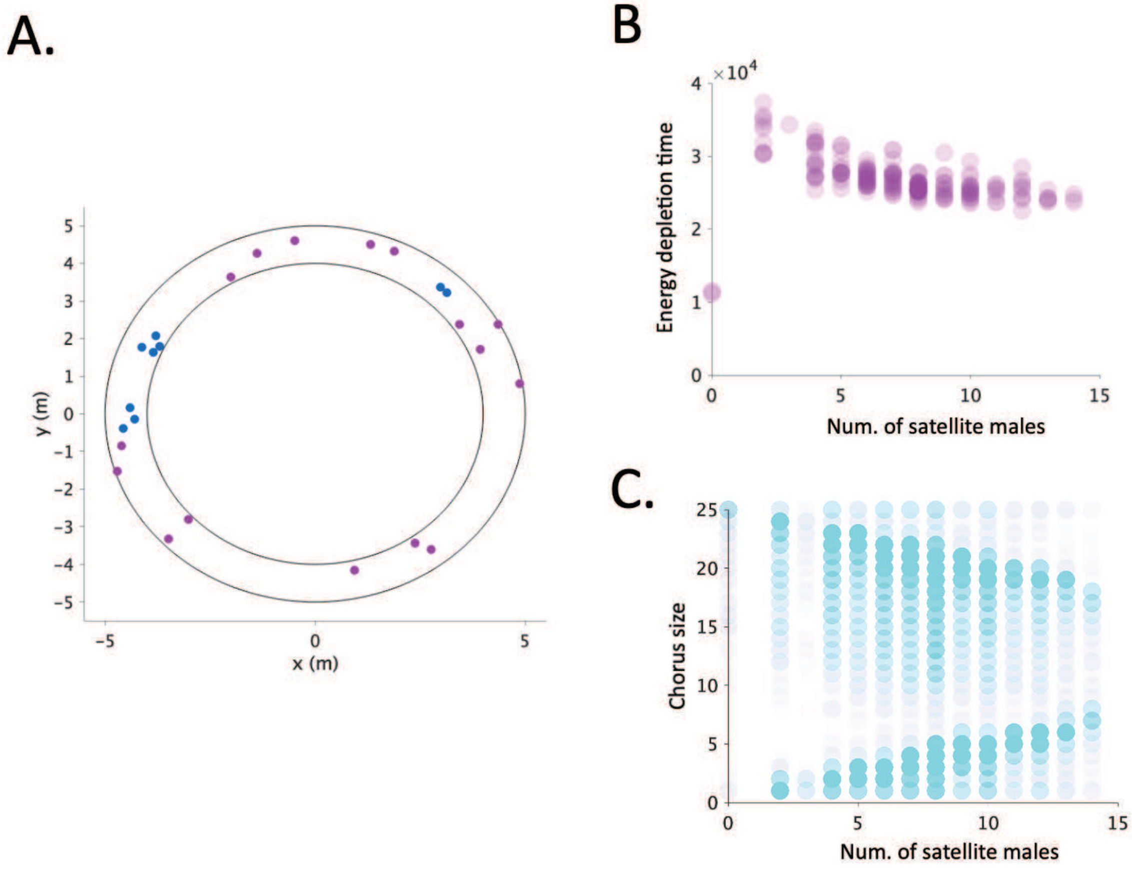


**Figure S1.** Numerical simulation on a large aggregation with 25 model frogs that are slightly scattered along a circular field. (A) Representative spatial distribution of the model frogs. (B) The dependency of *energy depletion time* on the number of satellite males. (C) The dependency of *chorus size* on the number of satellite males. We repeated the simulation 200 times in each aggregation with randomized initial conditions, and overlaid translucent plots in each graph.

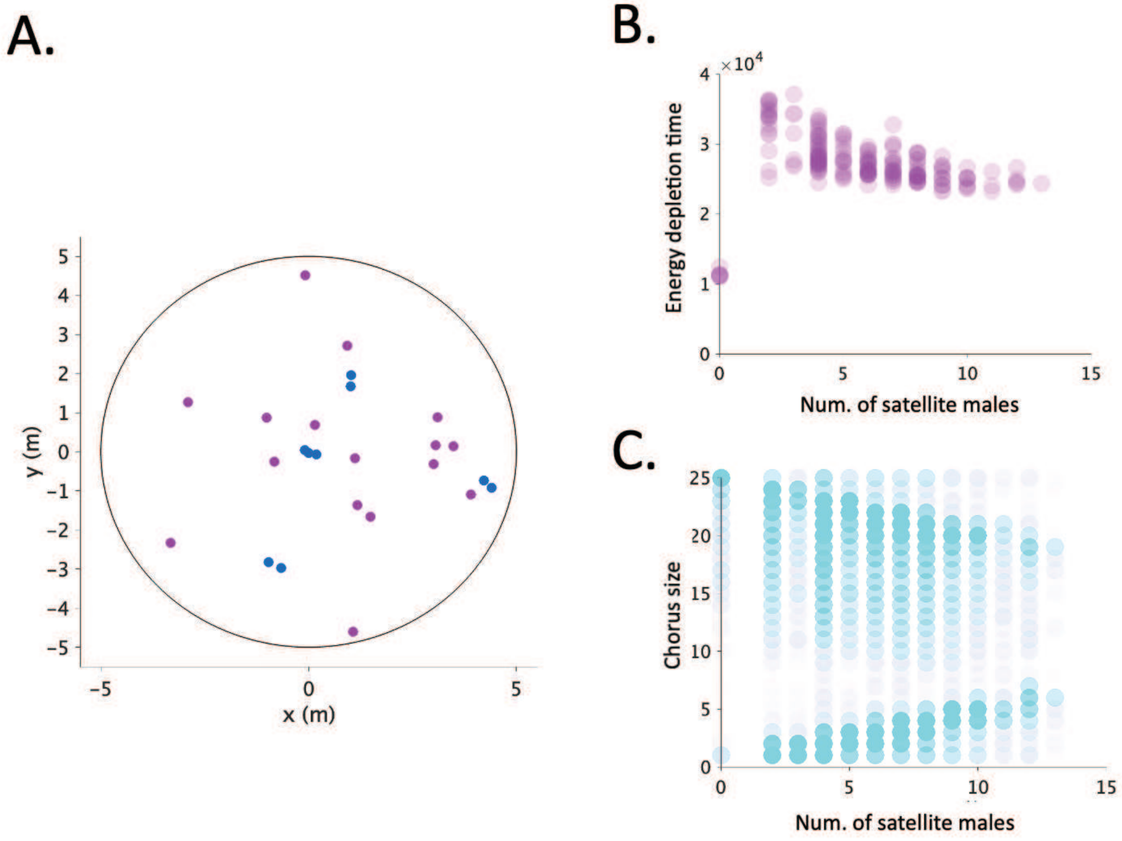


**Figure S2.** Numerical simulation on a large aggregation with 25 model frogs that are scattered within a circular field. (A) Representative spatial distribution of the model frogs. (B) The dependency of *energy depletion time* on the number of satellite males. (C) The dependency of *chorus size* on the number of satellite males. We repeated the simulation 200 times in each aggregation with randomized initial conditions, and overlaid translucent plots in each graph.

## References

[1] Aihara I, Kominami D, Hirano Y, Murata M (2019) Mathematical modelling and application of frog choruses as an autonomous distributed communication system. Royal Society Open Science 6: 181117.

[2] Gerhardt HC, Huber F (2002) Acoustic communication in insects and anurans. Chicago: University of Chicago Press.
